# Supplementary material for: Query-Dependent Video Representation for Moment Retrieval and Highlight Detection
Source: arXiv:2303.13874 source file (2023-03-24)
Supplement: Supplementary file 1 [file supplementary.tex]

% CVPR 2023 Paper Template
% based on the CVPR template provided by Ming-Ming Cheng (https://github.com/MCG-NKU/CVPR_Template)
% modified and extended by Stefan Roth (stefan.roth@NOSPAMtu-darmstadt.de)

\documentclass[10pt,twocolumn,letterpaper]{article}

%%%%%%%%% PAPER TYPE  - PLEASE UPDATE FOR FINAL VERSION
% \usepackage[review]{cvpr_supp}      % To produce the REVIEW version
\usepackage{cvpr}              % To produce the CAMERA-READY version
%\usepackage[pagenumbers]{cvpr} % To force page numbers, e.g. for an arXiv version

% Include other packages here, before hyperref.
\usepackage{graphicx}
\usepackage{amsmath}
\usepackage{amssymb}
\usepackage{booktabs}

%------ Ours ------%
\usepackage{array,multirow,graphicx}
\usepackage{float}
\usepackage{amsmath}
\usepackage{mathtools}
\usepackage{bbm}
\usepackage{hhline}
\usepackage{boldline}
\usepackage{tabularx}
\usepackage{comment}
\usepackage{color}
\usepackage{amssymb}
\usepackage{booktabs}
\usepackage{hhline}
\usepackage{multicol}
\usepackage{microtype}      % microtypography
\usepackage{xcolor}         % colors
\usepackage{hhline}%#######
\usepackage{bbm}
\usepackage{boldline}
\usepackage{amssymb}
\usepackage{algorithm}
\usepackage{algpseudocode}
\usepackage{pifont}% http://ctan.org/pkg/pifont
\usepackage{soul} %\st
\usepackage{subcaption}
\usepackage{caption}

% It is strongly recommended to use hyperref, especially for the review version.
% hyperref with option pagebackref eases the reviewers' job.
% Please disable hyperref *only* if you encounter grave issues, e.g. with the
% file validation for the camera-ready version.
%
% If you comment hyperref and then uncomment it, you should delete
% ReviewTempalte.aux before re-running LaTeX.
% (Or just hit 'q' on the first LaTeX run, let it finish, and you
%  should be clear).
\usepackage[pagebackref,breaklinks,colorlinks]{hyperref}
\usepackage{lipsum}

% Support for easy cross-referencing
\usepackage[capitalize]{cleveref}

\crefname{section}{Sec.}{Secs.}
\Crefname{section}{Section}{Sections}
\Crefname{table}{Table}{Tables}
\crefname{table}{Tab.}{Tabs.}

%%%%%%%%% PAPER ID  - PLEASE UPDATE
 % *** Enter the CVPR Paper ID here

\newcommand{\Skip}[1]{}

\begin{document}

%%%%%%%%% TITLE - PLEASE UPDATE
% \title{Cross-Modal Conditioning: Query-Dependent DETR \\ for Moment Retrieval and Highlight Detection}
% \title{
% Appendix for 
% ``Query-Dependent Video Representation \\ for Moment Retrieval and Highlight Detection''
% }
\title{
Appendix for 
``\textit{Query-Dependent Video Representation \\ for Moment Retrieval and Highlight Detection}''
}

\author{
WonJun Moon$^{1,\ast}$, Sangeek Hyun$^{1,\ast}$, SangUk Park$^{2}$, Dongchan Park$^{2}$, Jae-Pil Heo$^{1,\star}$\\
$^{1}$Sungkyunkwan University, $^{2}$Pyler\\
{\tt\small \{wjun0830, hsi1032, jaepilheo\}@g.skku.edu,} {\tt\small \{psycoder, cto\}@pyler.tech}
}

\maketitle
\newcommand{\mc}[3]{\multicolumn{#1}{#2}{#3}}

\input{sup_1_trainingdetail}
\input{sup_2_querylength}

%%%%%%%%% BODY TEXT

%%%%%%%%% REFERENCES
{\small
\bibliographystyle{ieee_fullname}
\bibliography{egbib}
}

\end{document}
